# Supplementary material for: Learning and Planning for Temporally Extended Tasks in Unknown Environments
Source: arXiv:2104.10636 source file (2021-04-28)
Supplement: Supplementary file 1 [file appendix.tex]

\subsection{Computing cost using Monte-Carlo Sampling}
\label{sub:mcts}
Exhaustive search is impractical for a problem of this complexity. Fortunately however, it is not necessary. We have structured our learning problem such that, given a subgoal as an input, our network estimates the probability that the action succeeds, as well as the cost of that action for either outcome. This is discussed further is section \ref{sec:learning}. With this model, we use Monte-Carlo sampling methods to simulate the long-term outcomes and costs of sequences of actions.

\gls{mcts} is a probabilistic sampling technique which allows the agent to to greatly reduce the complexity of the cost calculation by ignoring low probability regions in the policy tree which do not contribute in a meaningful way to cost of the policy. Traditionally, \gls{mcts} relies on a state-based representation which does not need to keep track of the history of actions in a plan. Since the subgoals available to our agent depend on previous actions in a proposed sequence however, \gls{pouct} as presented by Silver and Veness \cite{POMCP} is better suited for our application. 

\gls{pouct} is a generalization of the \gls{mcts} approach, which keeps track of histories of actions and outcomes. The nodes of our search tree correspond to belief states $b_\hist$, and each node contains a value $V(b_\hist,a)$, and a visitation count $N(b_\hist,a)$. The procedure for growing and refining a \gls{pouct} tree is to begin at the root node ($b_{\hist_0}$), and pick the most promising action according to:
\begin{equation}\label{eq:po-uct}
V(b_\hist,a)^* = V(b_\hist,a) + c\sqrt{\frac{log(N(b_\hist))}{N(b_\hist,a)}},
\end{equation}
where $N(b_\hist)$ corresponds to the number of time we have seen that node in simulations, and $N(b_\hist,a)$ is how often we have seen that node and chosen action $a$. The second term in the above equation captures the relative ratio of exploration and exploitation, and is modulated by the scalar $c$. One impact of this term is that all actions from a particular node are simulated at least once before any are tried a second time. 

Best first search according \eqref{eq:po-uct} will continue through the tree until a node has been selected which has not yet been simulated. From there, a sequence of actions is randomly selected according to some policy (often uniformly random) until either the agent simulates reaching an accepting state, or no actions are available and the robot fails (accruing some additional cost). This is called the rollout step, after which, all costs are propagated back up the tree to update the $V(b,a)$ and $N(b,a)$ values of parent nodes until the root is reached. \gls{pouct} is an anytime algorithm, so once a pre-defined amount of time has passed, we stop simulating, and the action with the highest $Q(b,a)$ from the root node is chosen. Additionally, like \gls{mcts}, \gls{pouct} is asymptotically optimal, meaning if we simulate for long enough, we should expect to return the optimal action according to \eqref{eq:ltl-subgoal-planning-equation}.

\gls{pouct} is particularly well suited to our problem for three reasons. First, it enables the agent to reuse computation by probabilistically averaging the values of child nodes according to how often the algorithm selected them. The most promising branches are explored most often, leading their inputs to be more highly valued.  Second it requires a generative model of the outcomes and costs of different actions, which we get from the neural network. Finally, the set of possible outcomes from our discrete actions is discrete and small (either a subgoal succeeds or it doesn't. Therefore, we don't suffer from the infinitely large branching factors partially observable problems usually face in continuous domains.
